# Supplementary material for: System-level thermal and electrical modeling of battery systems for electric aircraft design
Source: arXiv:2408.16494 source file (2024-08-29)
Supplement: Supplementary file 1 [file Appendices.tex]

\newpage
\section*{Appendix A: Cell specific heat capacity estimation}\label{sec:AppendixA}

Estimating the specific heat capacity of the battery cell is performed over a constant current discharge of 600 seconds. We assume that the energy lost escapes purely as Joule heat and we apply Joule's Law as
\begin{equation}
    P_\mathrm{joule} \approx I_\mathrm{cell}^2\cdot R_0
\end{equation}
where $I_\mathrm{cell}$ is the discharge current and $R_0$ is the internal battery resistance. During the 600 s discharge, we model the consumed energy as
\begin{equation}
    {Q}(t) = -\int_{0}^{600}U_\mathrm{cell}(t)\cdot I_\mathrm{cell}(t)~\mathrm{d}t
\end{equation}
where $U_\mathrm{cell}(t)$ is the cell's voltage. Next, we estimate the specific heat with
\begin{equation}
    c_\mathrm{p} = \frac{Q}{m_\mathrm{cell}\cdot(T_\mathrm{end}-T_0)},
\end{equation}
where $m_\mathrm{cell}$ is the cell's mass, and $T_\mathrm{end}-T_0$ define the temperature difference of the cell. For the NMC in this work, this results in a $c_\mathrm{p}$ value of 1035 J/kg$\cdot$K.

\section*{Appendix B: HPPC test protocol}
At each 10\% state of charge increment, we start a pulse consisting of discharge, rest, and charge. The test assumes that the SOC does not change within the HPPC window at every pulse increment. The followed steps are as follows:
\begin{enumerate}
    % \item Discharge pulse at 1C for 10 seconds.
    % \item Rest for 40 seconds.
    % \item Charge pulse at 0.75C for 10 seconds.
    % \item Rest for 30 minutes.
    % \item Rest for 1 hour.
    % \item new
    \item Standard Constant Current - Constant Voltage (CCCV) charge to $U_\mathrm{cell,max}$.
    \item Rest for 1 hour.
    \item Constant Current (CC) discharge at 1 $\mathrm{C}$ for 30 seconds.
    \item Rest for 40 seconds.
    \item Charge pulse at 0.75 $\mathrm{C}$ for 10 seconds.
    \item Discharge at 1 $\mathrm{C}$ for 6 minutes.
    \item Rest for 1 hour.
    \item Repeat steps (3) - (7) 10 times.
\end{enumerate}
\vspace{12pt}

\begin{table}[ht]
\section*{Appendix C}
\centering
\caption{Aircraft and powertrain parameters and requirements.}
\label{tab:aircraftpara}
% \resizebox{\columnwidth}{!}{%

\begin{tabular}{l|l|c|l}
Symbol &  Property               &  Value   &  Units \\ \hline
  &   &   &  \vspace{-7pt} \\ 
    $m_\mathrm{empty}$  &  Empty aircraft mass &     1489     &kg        \\
    $m_\mathrm{max}$  &  Maximum aircraft mass &     3000     &kg        \\
      $S_\mathrm{w}$ &  Wing area              &  20.8        &  m$^2$      \\
      $C_\mathrm{l}$ &  Lift coefficient       &    0.85      &  -      \\
$C_\mathrm{d}$ & Drag coefficient        & 0.03            &  -\\
$\alpha_\mathrm{max}$ & Maximum angle of attack & 4           & $^\circ$ \\
$\gamma_\mathrm{max}$ & Maximum flight path angle & 8           & $^\circ$ \\
$\gamma_\mathrm{min}$ & Minimum flight path angle & -1           & $^\circ$ \\
$n_\mathrm{m}$ & Number of motors        &  2           & - \\
$P_\mathrm{m,max}$ & Maximum motor power     &   250        & kW \\
$\eta_\mathrm{p}$ & Propeller efficiency    &   0.71          & -\\
 $\omega_\mathrm{p,cons}$& Constant propeller speed    & 4000 & rpm\\
 $\zeta_{\mathrm{b,max}}$ & Maximum SOC    &  1          & - \\
   $\zeta_{\mathrm{b,min}}$ &  Minimum SOC    &  0.15           & - \\
      $P_{\mathrm{aux}}$ &  Auxiliary power consumption    &  4           & kW \\
       % $s_\mathrm{min}$  & Minimal flight range    &  400           & km \\
\end{tabular}%
% }
\end{table}

\begin{table}[ht]
\section*{Appendix D}
\centering
\caption{Cell parameters.}
\label{tab:cellpara}
% \resizebox{\columnwidth}{!}{%

\begin{tabular}{l|l|c|l}
Symbol              & {\color[HTML]{000000} Property}               & {\color[HTML]{000000} Value} & {\color[HTML]{000000} Units}    \\ \hline
&   &   &  \vspace{-6pt} \\ 
$Q_\mathrm{cell}$   & {\color[HTML]{000000} Capacity}               & {\color[HTML]{000000} 11.84} & {\color[HTML]{000000} Ah}       \\
$U_\mathrm{cell,max}$    & {\color[HTML]{000000} Maximum voltage}        & {\color[HTML]{000000} 4.2}   & {\color[HTML]{000000} V}        \\
$U_\mathrm{cell,nom}$    & {\color[HTML]{000000} Nominal voltage}        & {\color[HTML]{000000} 3.4}   & {\color[HTML]{000000} V}        \\
$U_\mathrm{cell,min}$    & {\color[HTML]{000000} Minimum voltage}        & {\color[HTML]{000000} 2.5}   & {\color[HTML]{000000} V}        \\
$I_\mathrm{ch,max}$ & {\color[HTML]{000000} Maximum charge current} & {\color[HTML]{000000} 2.32}  & {\color[HTML]{000000} A}        \\
$I_\mathrm{dis,max}$ & {\color[HTML]{000000} Maximum discharge current}  & {\color[HTML]{000000} 34.8} & {\color[HTML]{000000} A}     \\
$T_\mathrm{cell,min}$    & {\color[HTML]{000000} Minimum temperature}    & {\color[HTML]{000000} -20}   & {\color[HTML]{000000} $^\circ$C} \\
$T_\mathrm{cell,max}$    & {\color[HTML]{000000} Maximum temperature}    & {\color[HTML]{000000} 55}    & {\color[HTML]{000000} $^\circ$C} \\
$T_\mathrm{cell,opt}$    & {\color[HTML]{000000} Optimal temperature range}    & {\color[HTML]{000000} [15,35]}    & {\color[HTML]{000000} $^\circ$C} \\
$m_\mathrm{cell}$    & {\color[HTML]{000000} Cell mass} & {\color[HTML]{000000} 0.103}  & {\color[HTML]{000000} kg} \\
$\rho_\mathrm{GED}$    & {\color[HTML]{000000} Gravimetric energy density} & {\color[HTML]{000000} 390}  & {\color[HTML]{000000} Wh/kg} \\
$c_\mathrm{p}$    & {\color[HTML]{000000} Specific heat capacity} & {\color[HTML]{000000} 1035}  & {\color[HTML]{000000} J/(kg$\cdot$K)} \\
$\operatorname{Bi}$    & {\color[HTML]{000000} Biot number} & {\color[HTML]{000000} 0.0367}  & {\color[HTML]{000000} -} \\
\end{tabular}%
% }
\end{table}

\begin{table}[ht]
\section*{Appendix E}
\centering
\caption{Applied BTMS values.}
\label{tab:BTMSval}
\resizebox{\columnwidth}{!}{%

\begin{tabular}{l|l|c|c|l}
Symbol              & {\color[HTML]{000000} Property}               & {\color[HTML]{000000} Value air} & {\color[HTML]{000000} Value water} & {\color[HTML]{000000} Units}    \\ \hline
      &   &   &   &  \vspace{-6pt} \\ 
$T_\mathrm{fl,in}$   & {\color[HTML]{000000} Inlet temperature}               & {\color[HTML]{000000} 20}  & {\color[HTML]{000000} 20}& {\color[HTML]{000000}$^\circ$C}       \\
$w_\mathrm{ch}$ & {\color[HTML]{000000} Channel width} & {\color[HTML]{000000} $3 \cdot 10^{-3}$} & {\color[HTML]{000000} $3 \cdot 10^{-3}$} & {\color[HTML]{000000} m} \\
$\dot{V}_\mathrm{fl,max}$    & {\color[HTML]{000000} Maximum flow rate}        & {\color[HTML]{000000} 0.0625}& {\color[HTML]{000000} 0.0045}    & {\color[HTML]{000000} m$^3$/s}        \\
$\nu_\mathrm{fl}$ & {\color[HTML]{000000} Kinematic viscosity} & {\color[HTML]{000000} $1.48 \cdot 10^{-5}$} & {\color[HTML]{000000} $1.002 \cdot 10^{-6}$} & {\color[HTML]{000000} m$^2$/s} \\
$k_\mathrm{fl}$    & {\color[HTML]{000000} Thermal conductivity}        & {\color[HTML]{000000} 30} & {\color[HTML]{000000} 600}   & {\color[HTML]{000000} W/K}        \\
$\rho_\mathrm{fl}$    & {\color[HTML]{000000} Density}        & {\color[HTML]{000000} 1.292} & {\color[HTML]{000000} 1000}  & {\color[HTML]{000000} kg/m$^3$}        \\
$c_\mathrm{p,fl}$    & {\color[HTML]{000000} Specific heat capacity}        & {\color[HTML]{000000} 1006}  & {\color[HTML]{000000} 4182}  & {\color[HTML]{000000} J/kg$\cdot$K}        \\
$\operatorname{Pr}$    & {\color[HTML]{000000} Prandtl number}         & {\color[HTML]{000000} 0.71} & {\color[HTML]{000000} 6.9}  & {\color[HTML]{000000} -}        \\
$l$ & Cooling channel length & 1.6 &1.6&m
\end{tabular}%
}
\end{table}

\begin{table}[ht]
\section*{Appendix F}
\centering
\caption{Battery system parameters without BTMS.}
\label{tab:batpara}
\resizebox{\columnwidth}{!}{%

\begin{tabular}{l|l|c|l}
Symbol & {\color[HTML]{000000} Property}              & {\color[HTML]{000000} Value} & {\color[HTML]{000000} Units}       \\ %\hline
\hline & & \\[-2ex]%!!!!!!!!!!!! 
       $U_\mathrm{b}$&Nominal battery system voltage&401.2&V\\
        $Q_\mathrm{b}$&Battery system capacity&304&kWh\\
       $m_\mathrm{b}$& \begin{tabular}[c]{@{}l@{}}Total battery system mass\\ \textit{(including 10\% cell-to-system weight)}\end{tabular} & {\color[HTML]{000000} 856}   & {\color[HTML]{000000} kg}          \\
       $\rho_\mathrm{GED,b}$ & \begin{tabular}[c]{@{}l@{}}Battery system energy density\\ \textit{(including 10\% cell-to-system weight)}\end{tabular} &  355&Wh/kg \\
      $P_\mathrm{b,max,dis}$& {\color[HTML]{000000} Maximum discharge power}        &912 & {\color[HTML]{000000} kW} \\
   $n_\mathrm{p}$ & {\color[HTML]{000000} Number of parallel cells}                       &  {\color[HTML]{000000} 64}     & {\color[HTML]{000000} -}\\
        $n_\mathrm{s}$& {\color[HTML]{000000} Number of series cells}                       &  {\color[HTML]{000000} 118}     & {\color[HTML]{000000} -} \\
        $\Delta T_\mathrm{cell,max}$&\begin{tabular}[c]{@{}l@{}}Maximum cell temperature\\difference in system\end{tabular}&5&$^\circ$C
\end{tabular}%
}
\end{table}

% \begin{figure}[h]
% \section*{Appendix G}
%     \centering
%     \includegraphics[width=0.9\linewidth]{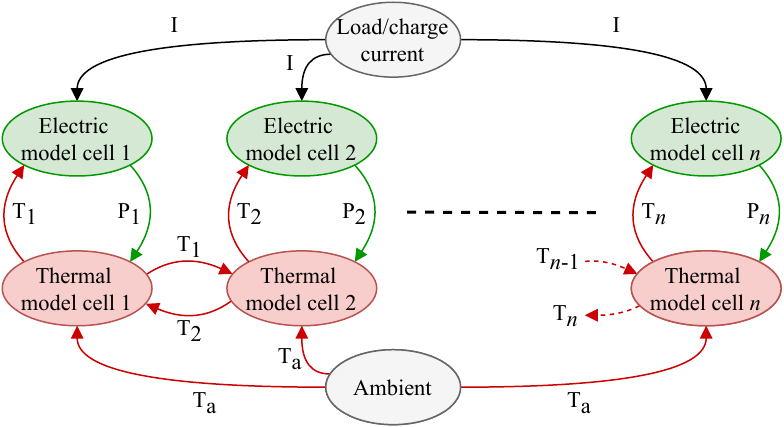}
%     \caption{Schematic representation of cells within thermo-electrical network.}
%     \label{fig:ThermalNodes}
% \end{figure}

\begin{figure}[h]
\section*{Appendix G}
    \centering
    \includegraphics[width=0.99\linewidth]{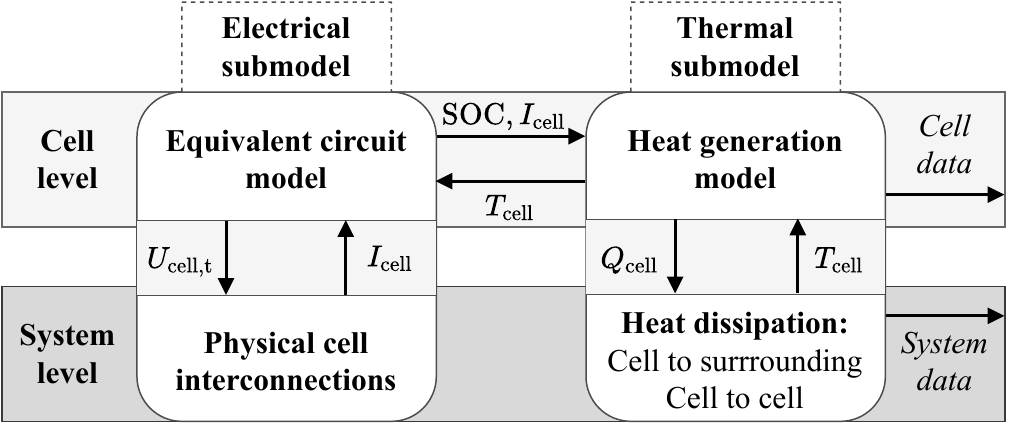}
    \caption{Cell vs. system modeling framework.}
    \label{fig:ThermalModeling}
\end{figure}
