# Supplementary material for: System-level thermal and electrical modeling of battery systems for electric aircraft design
Source: arXiv:2408.16494 source file (2024-08-29)
Supplement: Supplementary file 2 [file AppendicesEXT.tex]

\onecolumn
\section*{External appendices}\label{ch:AppExt}

\subsection{\ul{General cell parameters for 11.84 Ah NMC cell}}

\begin{table}[h]
\centering
% \resizebox{\columnwidth}{!}{%

\begin{tabular}{l|l|l|l}
Symbol              & {\color[HTML]{000000} Property}               & {\color[HTML]{000000} Value} & {\color[HTML]{000000} Units}    \\ \hline
-   & {\color[HTML]{000000} Cell chemistry}               & {\color[HTML]{000000} NMC} & {\color[HTML]{000000}-}       \\
$Q_\mathrm{cell}$   & {\color[HTML]{000000} Capacity}               & {\color[HTML]{000000} 11.84} & {\color[HTML]{000000} Ah}       \\
$U_\mathrm{max}$    & {\color[HTML]{000000} Maximum voltage}        & {\color[HTML]{000000} 4.2}   & {\color[HTML]{000000} V}        \\
$U_\mathrm{max}$    & {\color[HTML]{000000} Nominal voltage}        & {\color[HTML]{000000} 3.4}   & {\color[HTML]{000000} V}        \\
$U_\mathrm{max}$    & {\color[HTML]{000000} Minimum voltage}        & {\color[HTML]{000000} 2.5}   & {\color[HTML]{000000} V}        \\
$I_\mathrm{ch,max}$ & {\color[HTML]{000000} Maximum charge current} & {\color[HTML]{000000} 2.32}  & {\color[HTML]{000000} A}        \\
$I_\mathrm{dis,max}$ & {\color[HTML]{000000} Maximum discharge current}  & {\color[HTML]{000000} 34.8} & {\color[HTML]{000000} A}     \\
$T_\mathrm{min}$    & {\color[HTML]{000000} Minimum temperature}    & {\color[HTML]{000000} -20}   & {\color[HTML]{000000} $^\circ$C} \\
$T_\mathrm{max}$    & {\color[HTML]{000000} Maximum temperature}    & {\color[HTML]{000000} 55}    & {\color[HTML]{000000} $^\circ$C} \\
$\rho_\mathrm{VED}$    & {\color[HTML]{000000} Volumetric energy density}  & {\color[HTML]{000000} 797}  & {\color[HTML]{000000} Wh/l}  \\
$e_\mathrm{cell}$    & {\color[HTML]{000000} Specific energy}  & {\color[HTML]{000000} 1407.0}  & {\color[HTML]{000000} J/kg}  \\
$m_\mathrm{cell}$    & {\color[HTML]{000000} Cell mass} & {\color[HTML]{000000} 103.0}  & {\color[HTML]{000000} g} \\
$\rho_\mathrm{GED}$    & {\color[HTML]{000000} Gravimetric energy density} & {\color[HTML]{000000} 390}  & {\color[HTML]{000000} Wh/kg} \\
$l_\mathrm{cell}$    & {\color[HTML]{000000} Cell length} & {\color[HTML]{000000} 139.0}  & {\color[HTML]{000000} mm} \\
$h_\mathrm{cell}$    & {\color[HTML]{000000} Cell height} & {\color[HTML]{000000} 54.2}  & {\color[HTML]{000000} mm} \\
$w_\mathrm{cell}$    & {\color[HTML]{000000} Cell width} & {\color[HTML]{000000} 6.7}  & {\color[HTML]{000000} mm} \\
$c_\mathrm{p}$    & {\color[HTML]{000000} Specific heat capacity} & {\color[HTML]{000000} 1035}  & {\color[HTML]{000000} J/(kg$\cdot$K)} \\
$k$    & {\color[HTML]{000000} Thermal conductivity} & {\color[HTML]{000000} 26.5}  & {\color[HTML]{000000} W/(m$\cdot$K}) \\
% $h$    & {\color[HTML]{000000} Convective heat transfer coefficient} & {\color[HTML]{000000} \hl{xx}}  & {\color[HTML]{000000} W/(m$^2\cdot$K)} \\
\end{tabular}%
% }
\end{table}

\subsection{\ul{Figure: Cell ECM parameters obtained from HPPC fit}}

\begin{figure}[h]
\centering
\begin{subfigure}{.45\textwidth}
  \centering
  \includegraphics[width=\linewidth]{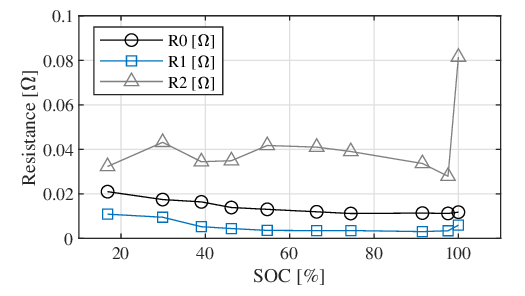}
  \caption{ECM resistance values}
  \label{fig:Rval}
\end{subfigure}%
\begin{subfigure}{.45\textwidth}
  \centering
  \includegraphics[width=\linewidth]{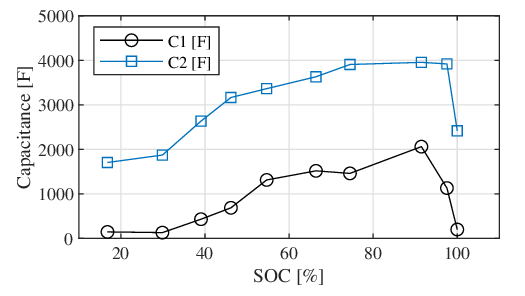}
  \caption{ECM capacitance values}
  \label{fig:Cval}
\end{subfigure}
% \caption{A figure with two subfigures}
\label{fig:RCvalues}
\end{figure}
% \begin{figure}[h]
%     \centering
%     \includegraphics[width=0.45\linewidth]{Figures/R_Values_SA03.eps}
%     \label{fig:R}
% \end{figure}
% \begin{figure}[h]
%     \centering
%     \includegraphics[width=0.45\linewidth]{Figures/C_Values_SA03.eps}
%     \label{fig:C}
% \end{figure}

\subsection{\ul{Figure: Battery discharge curve under different C-rates (specified by manufacturer)}}
\begin{figure}[h]
    \centering
    \includegraphics[width=0.5\linewidth]{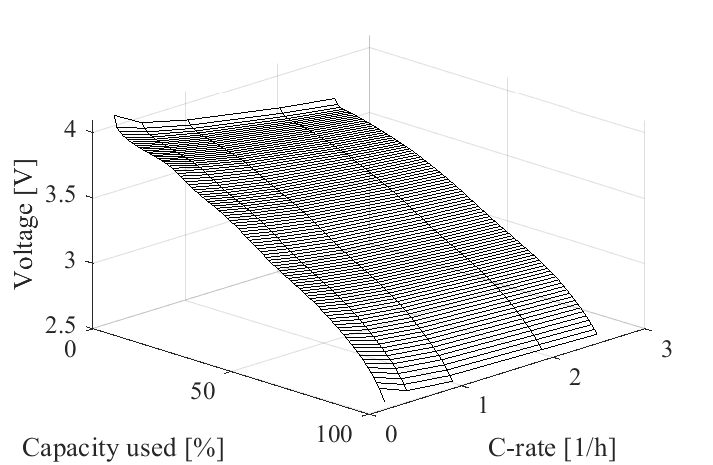}
    \label{fig:crates}
\end{figure}

\subsection{\ul{Flight profile sequence}}

% \subsection{\ul{Worst-case scenario: maximum power at low SOC}}

\subsection{\ul{Motor datasheet and efficiency map}}

% \subsection{\ul{Pump datasheet}}

% \subsection{\ul{Thermal runaway data fit}}

% \newpage
% \subsection{\ul{Code}}
% \begin{lstlisting}[style=Matlab-editor, basicstyle=\tiny]
% clc
% % close all
% % clear all
% clearvars t time
% % load load_cycles/load_cycle.mat

% BatPara = config.BatPara;
% SysPara = config.SysPara;

% %% Sim_battery_system in code
% dt                  = 1;%%%%%%%%%%%%%%%%%%%%%%%%%%%%%%%%%%%%%%%%%%%%%%%%%%%%%%%%%%%%%%%%%%%%%%0.02
% ns                  = SysPara.s_sys;% 3;
% np                  = SysPara.p_sys;% 6;
% startSOC            = 0.98;
% U_cell_start        = 4.135;        % 4.184;%11.88/3;

% Balancing.R         = SysPara.Balancing.R;      %33/np %% 33 Ohms
% Balancing.I_limit   = SysPara.Balancing.I_Limit;
% Balancing.U_delta   = SysPara.Balancing.U_Delta;
% Balancing.U_limit   = SysPara.Balancing.U_Limit;
% Balancing.t_start   = SysPara.Balancing.t_Start;

% m_cell              = BatPara.physical.m;
% cp_cell             = BatPara.thermal.c;
% A_cell              = BatPara.physical.A; % m2
% EnCo                = BatPara.thermal.EnCo;
% U_hys_enable        = 0;
% K_transfer          = results.SysPara.thermal.transfer.K_transfer;%SysPara.thermal.transfer.K_transfer;

% %% Cell parameters for 2RC Lookup tables 
% C_cell              = BatPara.electrical.C_A; %11;%Ah!!!
% T_amb               = 20;
% alpha_cell_ambient(:,:,1)      = 0*ones(np,ns);%5;%SysPara.thermal.alpha_cell_ambient;%%%%%%%%%%%%%%%%%%%%%%%%%%%%%%
% T_cell_ambient(:,:,1)      = 25*ones(np,ns);%results.SysPara.thermal.T_cell_ambient;%SysPara.thermal.T_cell_ambient;

% %% Create Parameter lookup grids (griddedInterpolant)
% %BatPara.electrical.dyn.R_0 %11x2x2: 11_soc*2_T*2_crate, but one dimension can be removed
% SOC_range           = BatPara.electrical.dyn.SOC;%0:0.1:1;
% T_range             = [25, 25.01];
% C_rate_range        = [-1,1];

% % R0_range          = squeeze(BatPara.electrical.dyn.R_0(:,1,:)); %remove 3rd dimension
% R0_range            = BatPara.electrical.dyn.R_0;
% R1_range            = BatPara.electrical.dyn.R1;
% C1_range            = BatPara.electrical.dyn.C1;
% R2_range            = BatPara.electrical.dyn.R2;
% C2_range            = BatPara.electrical.dyn.C2;

% % grid everything, or use interp2
% [SOCgrid,Tgrid,Cgrid] = ndgrid(SOC_range,T_range,C_rate_range); % create ndgrid
% R0_grid = griddedInterpolant(SOCgrid,Tgrid,Cgrid,R0_range);
% R1_grid = griddedInterpolant(SOCgrid,Tgrid,Cgrid,R1_range);
% C1_grid = griddedInterpolant(SOCgrid,Tgrid,Cgrid,C1_range);
% R2_grid = griddedInterpolant(SOCgrid,Tgrid,Cgrid,R2_range);
% C2_grid = griddedInterpolant(SOCgrid,Tgrid,Cgrid,C2_range);

% SOC_OCV_range   = BatPara.electrical.OCV.SOC;
% OCV_range       = BatPara.electrical.OCV.U;
% OCV_grid        = griddedInterpolant(SOC_OCV_range,OCV_range);

% U_hys_max_range = BatPara.electrical.OCV.U_hyst;
% U_hys_max_grid  = griddedInterpolant(SOC_OCV_range,U_hys_max_range);

% %% Preallocations
% I_cell(:,:,1)      = 0*ones(np,ns);
% SOC(:,:,1)         = min(max((startSOC + (0.005*randn(np,ns))), 0), 0.99);
% % SOC(:,:,1)         = startSOC*ones(np,ns);
% C_rate_cell(:,:,1) = 0*ones(np,ns);
% time(:,:,1)        = 0*ones(np,ns);
% U_hys(:,:,1)       = 0*ones(np,ns);
% U_RC1(:,:,1)       = 0*ones(np,ns);
% U_RC2(:,:,1)       = 0*ones(np,ns);
% I_bal(:,:,1)       = 0*ones(np,ns);
% I_pack(1)          = 0;

% U_cell(:,:,1)       = U_cell_start*ones(np,ns);
% U_pack(1)           = sum(U_cell(1,:,1));
% U_pot(:,:,1)        = 0*ones(np,ns);
% U_RC_sum(:,:,1)     = 0*ones(np,ns);
% U_R(:,:,1)          = 0*ones(np,ns);
% max_T_channel_out(1) = config.BTMSConfig.T_fluid;


% PQ_cell(:,:,1) = 0*ones(np,ns);

% T_cell(:,:,1)      = T_amb*ones(np,ns);
% % T_cell_amb         = T_cell_amb; % taken to be constant over flight cycle, 
% % could change with cooling system integrated
% PQ_cell_irr(:,:,1) = 0*ones(np,ns);
% PQ_cell_rev(:,:,1) = 0*ones(np,ns);
% PQ_ambient(:,:,1)  = 0*ones(np,ns);
% PQ_transfer(:,:,1) = 0*ones(np,ns);

% run('deviations_stat');

% m_cell  = m_cell.*SysPara.DeviationMap.m;
% cp_cell = cp_cell.*SysPara.DeviationMap.c;
% EnCo    = EnCo.*SysPara.DeviationMap.EnCo;




% %% BTMS inputs
% A_x = results.SysPara.thermal.transfer.A_x;
% A_y = results.SysPara.thermal.transfer.A_y;
% A_z = results.SysPara.thermal.transfer.A_z;

% T_fluid = config.BTMSConfig.T_fluid;
% Vdot_BTMS = config.BTMSConfig.Vdot_BTMS;
% BTMSConfig = config.BTMSConfig;

% %% %%%%%%%%%%%%%%%%%%%%%%%%%%%%%%%%%%%%%%%%%%%%%%%%%%%%%%%%%%%%%%%%%%%%%%%
% %% Functional code, main loop
% load('newCurrent.mat')
% I_load = -newCurrent/2; %*BatPara.electrical.C_A*np;
% t(1) = 0;
% disp('Starting cycle')
% tic
% for i = 2:1:length(I_load)

%     time = (i-1)*dt;
%     t(i) = time;
    
%     %R0_now = R0_grid(SOC,I_cell)
%     R0 = R0_grid(SOC(:,:,i-1),T_cell(:,:,i-1),C_rate_cell(:,:,i-1));
%     R1 = R1_grid(SOC(:,:,i-1),T_cell(:,:,i-1),C_rate_cell(:,:,i-1));
%     C1 = C1_grid(SOC(:,:,i-1),T_cell(:,:,i-1),C_rate_cell(:,:,i-1));
%     R2 = R2_grid(SOC(:,:,i-1),T_cell(:,:,i-1),C_rate_cell(:,:,i-1));
%     C2 = C2_grid(SOC(:,:,i-1),T_cell(:,:,i-1),C_rate_cell(:,:,i-1));
    
%     %% Statistical analysis
%     % disabled, enable if possible
%     R0 = R0.*SysPara.DeviationMap.R_0;
%     R1 = R1.*SysPara.DeviationMap.R1;
%     C1 = C1.*SysPara.DeviationMap.C1;
%     R2 = R2.*SysPara.DeviationMap.R2;
%     C2 = C2.*SysPara.DeviationMap.C2;

%     %% Electric potential for single cell (calculate the voltages)
%     % U_Potential = U_SOC + U_Hysteresis + U_RC1 + U_RC2
%     U_OCV = OCV_grid(SOC(:,:,i-1));
%     % Hysteresis from "Verbrugge, 2007 - Adaptive, multi-parameter battery 
%     % state estimator with optimized time weig
%     % hting factors"
%     U_hys_max   = U_hys_max_grid(SOC(:,:,i-1));
%     U_hys(:,:,i)    = (U_hys(:,:,i-1)+(dt.*I_cell(:,:,i-1).*...
%                         (U_hys_max-(U_hys(:,:,i-1).*sign(I_cell(:,:,i-1)))))).*U_hys_enable;
%     U_RC1(:,:,i)    = ((1-exp(-dt./(R1.*C1))).*R1.*I_cell(:,:,i-1)) +...
%                         (U_RC1(:,:,i-1).*(exp(-dt./(R1.*C1))));
%     U_RC2(:,:,i)    = ((1-exp(-dt./(R2.*C2))).*R2.*I_cell(:,:,i-1)) +...
%                         (U_RC2(:,:,i-1).*(exp(-dt./(R2.*C2))));
%     U_pot(:,:,i)    = U_RC1(:,:,i)+U_RC2(:,:,i)+U_OCV+U_hys(:,:,i);
%     U_RC_sum(:,:,i) = U_RC1(:,:,i)+U_RC2(:,:,i);
        
%     %% Ohmic voltage drop and compensating currents in parallel connections
%     I_pack = I_load(i);
%     U_cell(:,:,i)   = ones(np,1).*((sum(I_bal(:,:,i-1),1)+...
%         I_pack+sum((U_pot(:,:,i)./R0),1))./(sum((1./R0),1)));
%     U_R(:,:,i)      = U_cell(:,:,i)-U_pot(:,:,i);
%     I_cell(:,:,i)   = U_R(:,:,i)./R0;
    
%     %% Cell balancing
%     I_bal(:,:,i) = (-U_cell(:,:,i)/Balancing.R).*...
%         (time>=Balancing.t_start).*...
%         (abs(I_pack)<=Balancing.I_limit).*...33
%         (min(U_cell(:,:,i),[],"all")>=Balancing.U_limit).*...
%         ((U_cell(:,:,i)-min(U_cell(:,:,i),[],"all"))>Balancing.U_delta);
%         U_pack(i) = sum(U_cell(1,:,i));%Select and sum rows(series cells)
    
%     %% C-rate and SOC
%     C_rate_cell(:,:,i) = I_cell(:,:,i)/(C_cell*1);
%     delta_SOC = (I_cell(:,:,i)*dt)/(C_cell*3600);
%     SOC(:,:,i) = SOC(:,:,i-1) + delta_SOC;
    
%     %% Thermal model    
%     % Irreversible
%     % PQ_Cells,rev = - I_cell * T_cell * (dUocv/dT_cell) = - I_cell * T_cell * EnCo
%     % Eddahech et al (2013) Thermal characterization of a high-power
%     % lithium-ion battery
%     PQ_cell_irr(:,:,i) = abs(I_cell(:,:,i).*(U_RC_sum(:,:,i)+U_R(:,:,i)));
%     % Reversible
%     PQ_cell_rev(:,:,i) = -(I_cell(:,:,i).*EnCo.*T_cell(:,:,i-1));
%     PQ_cell(:,:,i) = PQ_cell_rev(:,:,i)+PQ_cell_irr(:,:,i);

%     %% BTMS input
%     % BTMSConfig.T_fluid
%     % BTMSConfig.Vdot_BTMS
%     tic
%     [max_T_channel_out(i), T_cell_ambient(:,:,i), alpha_cell_ambient(:,:,i)] =...
%         create_BTMS_input(T_cell(:,:,i-1), T_fluid, Vdot_BTMS,...
%         BTMSConfig, BatPara, A_x, A_y, A_z, ns, np);
%     toc

%     %% Lumped mass thermal model
%     % For fixed alpha_amb and T_cell_amb, enable code below:
%     % PQ_ambient(:,:,i) = alpha_cell_amb.*A_cell.*(T_cell_ambient-T_cell(:,:,i-1));
%     % T_cell(:,:,i) = T_cell(:,:,i-1)+((dt*(PQ_cell(:,:,i)+PQ_ambient(:,:,i)+...
%     % PQ_transfer(:,:,i-1)))./(m_cell.*cp_cell));
%     PQ_ambient(:,:,i) = alpha_cell_ambient(:,:,i).*A_cell.*(T_cell_ambient(:,:,i)-T_cell(:,:,i-1));
%     T_cell(:,:,i) = T_cell(:,:,i-1)+((dt*(PQ_cell(:,:,i)+PQ_ambient(:,:,i)+...
%         PQ_transfer(:,:,i-1)))./(m_cell.*cp_cell));

%     %% Heat transfer model
%     Heat_transfer = 1; %on/off
%     % K_transfer % Define a function to shape the K matrix
%     % reshape the matrix to display the parallel cells on the rows and series cells in columns.
%     PQ_transfer(:,:,i) = reshape((K_transfer*reshape(T_cell(:,:,i-1),[],1)),np,ns)*Heat_transfer;

    
%     %% Progress bar of model
%     if ~(mod(i,1000))
%     disp([num2str(i/length(I_load)*100),' %'])
%     end
% end
% toc
% return

% %% plots %%%%%%%%%%%%%%%%%%%%%%%%%%%%%%%%%%%%%%%%%%%%%%%%%%%%%%%%%%%%%%%%%
% %% Cell State-of-charges
% figure()
% Dim = size(SOC);
% SOC2 = reshape (permute(SOC, [3,2,1]), Dim(3), []);
% plot (SOC2); 
% title('Cell State-of-charges')
% xlabel('Time [s]'); grid on
% return
% %% Battery system current load
% figure()
% plot(t,I_load)
% title('Battery system current load')
% xlabel('Time [s]'); grid on
% %% Battery system voltage
% figure()
% plot(t,U_pack)
% title('Battery system voltage')
% xlabel('Time [s]'); grid on
% %% Cell current loads
% figure()
% Dim = size(I_cell);
% I_cell2 = reshape(I_cell,...
%     [length(I_cell(:,1,1))*length(I_cell(1,:,1)), length(I_cell(1,1,:))]);
% %reshape (permute(I_cell, [3,2,1]), Dim(3), []);
% plot (I_cell2); 
% title('Cell current loads')
% xlabel('Time [s]'); grid on
% %% Cell voltages
% figure()
% Dim = size(U_cell);
% U_cell2 = reshape (permute(U_cell, [3,2,1]), Dim(3), []);
% plot (U_cell2); 
% title('Cell voltages')
% xlabel('Time [s]'); grid on
% %% Cell State-of-charges
% figure()
% Dim = size(SOC);
% SOC2 = reshape (permute(SOC, [3,2,1]), Dim(3), []);
% plot (SOC2); 
% title('Cell State-of-charges')
% xlabel('Time [s]'); grid on
% %% Cell ECM sum
% figure()
% Dim = size(U_RC_sum);
% U_RC_sum2 = reshape (permute(U_RC_sum, [3,2,1]), Dim(3), []);
% plot (U_RC_sum2); 
% title('Cell ECM sum')
% xlabel('Time [s]'); grid on
% %% Cell ohmic voltage drops
% figure()
% Dim = size(U_R);
% U_Rb = reshape (permute(U_R, [3,2,1]), Dim(3), []);
% plot (U_Rb); 
% title('Cell ohmic voltage drops')
% xlabel('Time [s]'); grid on
% %% Cell temperatures
% figure()
% Dim = size(T_cell);
% T_cell2 = reshape (permute(T_cell, [3,2,1]), Dim(3), []);
% plot (t,T_cell2); 
% title('Cell temperatures')
% xlabel('Time [s]'); grid on
% hold on
% plot(t,max_T_channel_out)
% %% Ambient heat transfer
% figure()
% Dim = size(PQ_ambient);
% PQ_ambient2 = reshape (permute(PQ_ambient, [3,2,1]), Dim(3), []);
% plot (t,PQ_ambient2); 
% title('Ambient heat transfer')
% xlabel('Time [s]'); grid on

% %% Needed cooling power
% P_cool = -sum(PQ_ambient2');
% plot (P_cool); 

% %% Heat transfer between cells
% figure()
% Dim = size(PQ_transfer);
% PQ_transfer2 = reshape (permute(PQ_transfer, [3,2,1]), Dim(3), []);
% plot (PQ_transfer2); 
% title('Heat transfer between cells')
% xlabel('Time [s]'); grid on

% %% Plot all in 1 figure
% % % figure()
% % % return
% % % %% Plot all in 1 figure
% % % figlist=get(groot,'Children');
% % % newfig = figure;
% % % newfig.WindowState = 'maximized';
% % % tcl=tiledlayout(newfig,'flow');
% % % 
% % % for i = 1:numel(figlist)
% % %     figure(figlist(i));
% % %     ax=gca;
% % %     ax.Parent=tcl;
% % %     ax.Layout.Tile=i;
% % % end
% % % close(figlist)


% %% functions (if needed)
% function [max_T_channel_out, T_cell_ambient, alpha_cell_ambient] = create_BTMS_input(T_cell, T_fluid_BTMS, Vdot_BTMS, BTMSConfig, BatPara, A_x, A_y, A_z, s, p)
%     %% Transform T_cell to column vector
%     T_cell_vec = reshape(T_cell, [numel(T_cell),1]);
%     %% Some necessary variables
%     A_dir = [A_x, A_y, A_z];
%     A_cell_total = BatPara.physical.A;
%     %% Get average temperature of cells adjacent to the cooling channels
%     T_avg_cell_channel = NaN(BTMSConfig.num_channels, 1);
%     for ii = 1:BTMSConfig.num_channels
%         T_avg_cell_channel(ii) = sum(T_cell_vec(nonzeros(BTMSConfig.channel_def_mat(ii,:))'))/BTMSConfig.channel_num_adj_cells(ii);
%     end
%     %% Get volume and mass flow and speed through each cooling channel
%     %% Calculate channel heat transfer coefficient
%     %% Calculate average cooling channel temp
%     T_channel_out = NaN(BTMSConfig.num_channels, 1);
%     for ii = 1:BTMSConfig.num_channels
%         T_channel_out(ii) = get_fluid_out_temp(T_fluid_BTMS, T_avg_cell_channel(ii), BTMSConfig.channel_length(ii), BTMSConfig.channel_mdot(ii), BTMSConfig.fluid_para.cp, BTMSConfig.lambda_wall);
%     end
%     T_channel_avg = (T_fluid_BTMS + T_channel_out) / 2;
    
%     %% Write values is vectors
%     % T_cell_ambient_vec: Meat temperature around each cell
%     % alpha_cell_ambient_vec: Scaled heat transfer coefficient
%     [alpha_cell_ambient_vec, T_cell_ambient_vec]  = cal_output_vecs(T_channel_avg, BTMSConfig.channel_alpha, BTMSConfig.channel_def_mat, BTMSConfig.channel_orientation, A_dir, A_cell_total, s * p);
    
%     %% Recreate matrix structure for sim_battery_system
%     T_cell_ambient = reshape(T_cell_ambient_vec, [p, s]);
%     alpha_cell_ambient = reshape(alpha_cell_ambient_vec, [p, s]);
%     max_T_channel_out = max(T_channel_out);
% end

% function T_channel_out = get_fluid_out_temp(T_channel_in, T_avg_cell, channel_length, mdot, c_p_fluid, lambda_wall)
%     % Calculate approximated channel output temperature
%     % Approximation for axial flow in pipe
%         epsilon = lambda_wall / (mdot * c_p_fluid);
%     T_channel_out = (T_channel_in - T_avg_cell) * exp(-epsilon*channel_length) + T_avg_cell;  
        
% end

% function [alpha_cell_ambient_vec, T_cell_ambient_vec]  = cal_output_vecs(T_channel_avg, alpha_channel, channel_def_mat, channel_orientation, A_dir, A_cell_total, number_of_cells)
    
%     % Preallocate output vectors
%     alpha_cell_ambient_vec = zeros(1, number_of_cells);
%     T_cell_ambient_vec = zeros(1, number_of_cells);
    
%     for ii = 1:number_of_cells
        
%         % Look if a cell is adjacent to one or more cooling channels
%         [row, ~] = find(channel_def_mat == ii);
%             if length(row) >= 1     % Cell is in contact with one or more cooling channels
                
%                 % Calculate mean temperature around cell
%                 T_cell_ambient_vec(ii) = sum(T_channel_avg(row)) / length(row);
                
%                 % Get vector with area of heat transfers
%                 A_heat_total_cell = zeros(length(row), 1);
                
%                 x_dir = find(channel_orientation(row) == 'x');
%                 y_dir = find(channel_orientation(row) == 'y');
%                 z_dir = find(channel_orientation(row) == 'z');
                
%                 A_heat_total_cell(x_dir) = A_dir(1);
%                 A_heat_total_cell(y_dir) = A_dir(2);
%                 A_heat_total_cell(z_dir) = A_dir(3);
                
%                 % Calculate scaled heat transfer coefficient
                
%                 % The alpha value computed here will get multiplied with the total cell
%                 % surface in the simulation model --> We must scale the heat transfer
%                 % coefficient to the total cell surface.
    
%                 % Example for a cell that is cooled from both x-sides and from one y-side:
%                 % alpha_total = (alpha_x1*A_x + alpha_x2*A_x + alpha_y*A_y) / A_cell
                
%                 alpha_cell_ambient_vec(ii) = sum(alpha_channel(row) .* A_heat_total_cell) / A_cell_total;
            
%             end
%     end
% end


% \end{lstlisting}
